# Supplementary material for: Quantifying Hypothesis Space Misspecification in Learning from Human-Robot Demonstrations and Physical Corrections
Source: arXiv:2002.00941 source file (2020-02-28)
Supplement: Supplementary file 1 [file appendix2.tex]

\section{LogSumExp to avoid computational underflow}
\label{app:logsumexp}

In learning from demonstrations, computing some finite version of \eqref{eq:boltzmann} programatically can often times result in computational overflow or underflow. We demonstrate how to avoid these issues by employing the LogSumExp trick. 

The procedure transforms the equation of interest in logarithmic scale to begin with:

\begin{equation}
    \begin{aligned}
    %\log P(\xtraj_1,...,\xtraj_N \mid \weight,\beta) =& -\beta \weight^T \sum_{i=1}^N\trajfeat(\xtraj_i) -\\ 
%-& N \log \sum_{\bar{\xtraj}}e^{-\beta \weight^T \trajfeat(\bar{\xtraj})}. 
    \log P(\utraj_H \mid \state^0, \utraj_R; \weight,\beta) =& -\beta \cost_{\weight}(\xtraj,\utraj_R, \utraj_H) -\\
    -& \log \int_{\bar{\utraj}_H}e^{-\beta \cost_{\weight}(\bar{\xtraj}, \bar{\utraj}_R, \bar{\utraj}_H)} d\bar{\utraj}_H.
    \end{aligned}
    \label{eq:log_obs}
\end{equation}

The second term can be rewritten as:

\begin{equation}
    \begin{aligned}
    \log \int_{\bar{\utraj}_H}e^{-\beta \cost_{\weight}(\bar{\xtraj}, \bar{\utraj}_R, \bar{\utraj}_H)}d\bar{\utraj}_H = A + \log\int_{\bar{\utraj}_H}e^{-\beta \cost_{\weight}(\bar{\xtraj}, \bar{\utraj}_R, \bar{\utraj}_H)-A}d\bar{\utraj}_H . 
    \end{aligned}
\end{equation}

%\begin{equation}
%    \begin{aligned}
%    \log \sum_{\bar{\xtraj}}e^{-\beta \weight^T \trajfeat(\bar{\xtraj})} = A + \log \sum_{\bar{\xtraj}}e^{-\beta \weight^T \trajfeat(\bar{\xtraj})-A} . 
%    \end{aligned}
%\end{equation}

where $A = \max_{\bar\utraj} (-\beta \cost_{\weight}(\bar{\xtraj}, \bar{\utraj}_R, \bar{\utraj}))$, the maximum of all the exponents in the sum. By subtracting the maximum from all the exponents, we manage to avoid the computational overflow that is so common is exponentiation. Once we compute the logarithm of the sum, we can replace it in the above \eqref{eq:log_obs} and exponentiate the result to get the final answer.
